# Supplementary material for: Real-time Battery State of Charge and parameters estimation through Multi-Rate Moving Horizon Estimator
Source: arXiv:2310.14332 source file (2023-10-22)
Supplement: Supplementary file 1 [file appendix.tex]

\appendix
\section{A summary of Latin grammar}    % Each appendix must have a short title.
\section{Some Latin vocabulary}              % Sections and subsections are supported  
                                                                         % in the appendices.
